# Supplementary material for: How do ionic superdiscs self-assemble in nanopores?
Source: arXiv:2401.12663 ancillary file (2024-01-23)
Supplement: Supplementary file 1 [file ILC_ACSnano_SI.pdf]

# Supplementary Information: How do ionic superdiscs self-assemble in nanopores?

Zhuoqing Li,[†,‡,¶] Aileen R. Raab,[§] Mohamed A. Kolmangadi,[‖] Mark Busch,[†,‡,¶] Marco Grunwald,[§] Felix Demel,[§] Florian Bertram,[⊥] Andriy V. Kityk,[#] Andreas Schönhals,[‖] Sabine Laschat,[§] and Patrick Huber[*,†,‡,¶]

†*Institute for Materials and X-Ray Physics, Hamburg University of Technology, Denickestr. 15, 21073 Hamburg, Germany*

‡*Centre for X-Ray and Nano Science CXNS, Deutsches Elektronen-Synchrotron DESY, Notkestr. 85, 22607 Hamburg, Germany*

¶*Center for Hybrid Nanostructures CHyN, Hamburg University, Luruper Chaussee 149, 22761 Hamburg, Germany*

§*Institut für Organische Chemie, Universität Stuttgart, Pfaffenwaldring 55, 70569 Stuttgart, Germany*

‖*Bundesanstalt für Materialforschung und -prüfung (BAM), Unter den Eichen 87, 12205 Berlin, Germany*

⊥*Deutsches Elektronen-Synchrotron DESY, Notkestr. 85, 22607 Hamburg, Germany*

#*Faculty of Electrical Engineering, Czestochowa University of Technology, Al. Armii Krajowej 17, 42-200 Czestochowa, Poland*

E-mail: patrick.huber@tuhh.de

Phone: +49 40 42878-4545

# Gerneral Methods

All chemicals were used without further purification unless otherwise stated. Chromatography eluents (acetone, dichloromethane, light petroleum and ethyl acetate EtOAc) were distilled before use. $^{1}$H NMR spectra were measured using Bruker Avance 500 and Bruker Avance 700 spectrometers at 400 MHz and 500 MHz and $^{13}$C NMR spectra at 101 MHz and 126 MHz. COSY, HSQC and HMBC measurements were performed to assign the signals of the 1H and $^{13}$C NMR spectra. FT-IR spectra were measured on a Bruker Vektor 22 with an MKII Golden Gate single reflection diamond ATR. Absorption bands were rounded to integer wave numbers / $cm^{-1}$ and absorption intensities were classified as follows: w (weak), m (moderate), s (strong), vs (very strong). Mass spectra (MS) and high resolution mass spectra (HRMS) were measured by electrospray ionisation (ESI) using a Bruker MicrOTOF-Q spectrometer and by electron ionisation (EI) using an Exactive Plus Orbitrap mass spectrometer. Thin-layer chromatography was performed on Macherey-Nagel silica gel 60 F254 glass plates (thickness 0.20 mm) on aluminium (pore size 60 Å). Column chromatography was performed on Macherey-Nagel silica gel (particle diameter 40 - 60 µm).

# ILC Syntheses

The following compounds were synthesised from the literature: tetramethylguanidinium chloride,[1] Boc-DOPA(14,14,14),[1] DOPA(14,14,14),[1] Ac14.[1]

## General Procedures

### General procedure for alkylation of Boc exemplified by Boc-DOPA-(12,12,12) (GP 1)[2]

Acetonitrile (250 mL) was degassed for 30 min. L-3,4-dihydroxyp-henylalanine (2.44 g, 8.20 mmol), sodium iodide (0.17 g, 1.1 mmol) and potassium carbonate (8.06 g, 58.3 mmol) were added under a nitrogen atmosphere and stirred under reflux for 1 h. 1-Bromododecane (8.0 mL, 33.3 mmol) was added and the reaction mixture was stirred under reflux for 5 d. After filtering off the inorganic reactants, the solvent was removed under reduced pressure. The crude product was purified by column chromatography (SiO2, 50:1→30:1→5:1 PE/EE) to give a white solid (74 %, 4.85 g, 6.05 mmol).

### General procedure for the deprotection of the N-Boc protected alkylated amino acids exemplified by DOPA-(12,12,12) (GP 2)

Boc-DOPA (0.40 g, 0.50 mmol) was dissolved in dichloromethane (10 mL). Trifluoroacetic acid (0.40 mL, 5.2 mmol) was added and the reaction was stirred for 18 h. More dichloromethane (10 mL) was added and the reaction mixture was neutralised with Amberlyst 21. The base was filtered off and the solvent was removed under reduced pressure to give the product as a white solid in quantitative yield (356 mg, 0.50 mmol) without further purification.

### General procedure for the introduction of the guanidinium headgroup to the alkylated DOPA motif exemplified by Cy12 (GP 3)

DOPA-(12,12,12) (2.00 g, 2.85 mmol) and anhydrous $NaHCO_3$ (2.39 g, 28.5 mmol) were added to 30 mL of dry dichloromethane under a nitrogen atmosphere. A 1 M solution of 2-chloro-1,3-dimethyl-4,5-dihydro-1H-imidazol-3-ium chloride in dry dichloromethane (3.7 mL, 3.7 mmol) was slowly added and the reaction mixture was refluxed for 2 h. The inorganic reactant was filtered

off and the solution was acidified to pH = 1 with concentrated hydrochloric acid. The solvent was removed and the crude product was purified by column chromatography ($SiO_2$, 15:1) to give a colourless solid (51%, 1.20 g, 1.44 mmol).

## Syntheses

### Boc-DOPA

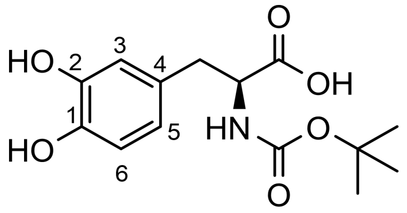


$C_{14}H_{19}NO_6$
(297.31)

Analogous to Rosen[3] L-3,4-dihydroxyphenylalanine (0.50 g, 2.54 mmol) and di-tert-butyldicarbonate (0.84 g, 3.84 mmol) were dissolved in 20 ml of an acetone/water mixture (V/V=1:1). Triethylamine (0.6 mL, 4.31 mmol) was added and the mixture was stirred for 24 h at room temperature. Saturated $NaHCO_3$-solution (20 mL) was added to the mixture, which was subsequently extracted with 2 X 25 mL EE. The aqueous phase was acidified to pH = 1 using concentrated hydrochloric acid and extracted with 3 x 40 mL EE. The organic phase was washed with brine (60 mL) and dried over $MgSO_4$. The solvent was removed under reduced pressure to yield the product as off-white to brown solid (97%, 0.73 mg, 2.46 mmol,); $^1$H NMR (400 MHz, DMSO-d$^6$): $\delta$ = 1.25–1.40 (m, 9H, $C(CH_3)_3$), 2.56–2.66 (m, 1H, $ArCH_2$), 2.73–2.82 (m, 1H, $ArCH_2$), 3.90–4.04 (m, 1H, NHCH), 6.41–6.47 (m, 3H,), 6.55–6.61 (m, 1H, 5-H), 6.89 (d, J = 8.2 Hz, 1H, 6-H), 8.62–8.70 (m, 1H, OH) ppm; $^{13}$C NMR (101 MHz, DMSO-d$^6$): $\delta$ = 28.2 ($C(CH_3)_3$), 35.9 ($ArCH_2$), 55.5 (HNCH), 78.1 ($C(CH_3)_3$) 115.3(C-6), 116.5 (C-3), 119.8 (C-5), 128.7 (C-4), 143.8 (C-1), 144.9 (C-2), 155.5 (N(CO)), 173.8 ((CO)) ppm.

**Boc-DOPA-(12,12,12)**

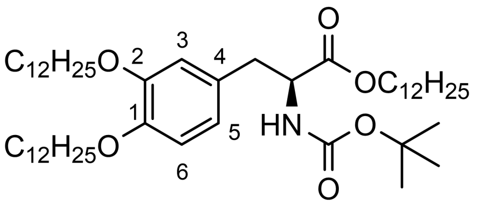


$C_{50}H_{91}NO_6$
(802.28)

Synthesis according to GP1; Boc-DOPA (2.44 g, 8.20 mmol), sodium iodide (0.17 g, 1.1 mmol), potassium carbonate (8.06 g, 58.3 mmol), 1-bromododecane (8.0 mL, 33 mmol), acetonitrile (250 mL); purification: column chromatography on silica gel (PE / EE 50 / 1 $\rightarrow$ 30 / 1 $\rightarrow$ 5 / 1); yield: white solid (74 %, 4.85 g, 6.05 mmol). $^1$H NMR (400 MHz, $CDCl_3$): $\delta$ = 0.88 (t, J = 6.6 Hz, 9H, $CH_3$), 1.21–1.39 (m, 50H, $CH_2$), 1.39–1.51 (m, 13H, $CH_2CH_2CH_2OAr$, $C(CH_3)_3$), 1.54–1.64 (m, 2H, $CH_2CH_2$-O-(CO)) 1.74–1.86 (m, 4H, $CH_2CH_2OAr$), 2.98–3.03 (m, 2H, $ArCH_2$), 3.90–3.99 (m, 4H, $CH_2OAr$), 4.08 (t, J = 6.7 Hz 2H, $CH_2$-O-(CO)), 4.48–4.55 (m, 1H, CHNH), 4.94 (d, J = 8.3 Hz, 1H, NH), 6.59–6.66 (m, 2H, 3-H, 5-H), 6.78 (d, J = 8.0 Hz, 1H, 6 H) ppm; $^{13}$C NMR (101 MHz, $CDCl_3$): $\delta$ = 14.3 ($CH_3$), 22.8, 26.0, 26.2, 26.2 ($CH_2$), 28.5 ($C(CH_3)_3$), 28.7, 29.4, 29.5, 29.6, 29.6, 29.7, 29.8, 29.8, 32.1 ($CH_2$), 38.0 ($ArCH_2$), 54.7 (HNCH), 65.6 ((CO)-$OCH_2$), 69.5, 69.5 ($OCH_2$), 79.9 ($C(CH_3)_3$), 114.2 (C-6), 115.3 (C-3), 121.8 (C-5), 128.7 (C-4), 148.4 (C-1), 149.3 (C-2), 155.2 (N(CO)), 172.2 ((CO)) ppm; FT-IR (ATR): $\tilde{\nu}$ = 3345 (w), 2917 (vs), 2849 (vs), 1733 (m), 1691 (vs), 1589 (w), 1531 (s), 1517(s), 1467 (m), 1428 (w), 1390 (w), 1368 (w), 1341 (w), 1322 (w), 1259 (s), 1233 (s), 1167 (vs), 1137 (s), 1058 (m), 849 (w), 795 (m), 722 (w), 672 (w) $cm^{-1}$; MS(EI): m/z for $C_{50}H_{91}NO_6$ calc.: 801.6846 [M], found: 802; HRMS(EI): m/z for $C_{50}H_{91}NO_6$ calc.: 801.6846 $[M]^+$, found: 801.6841.

**Boc-DOPA-(16,16,16)**

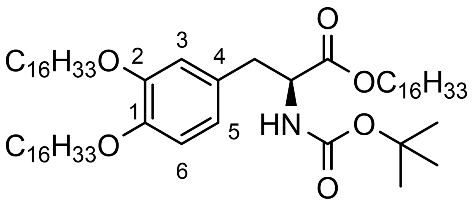


$C_{62}H_{115}NO_6$
(970.60)

Synthesis according to GP1; Boc-DOPA (2.04 g, 6.87 mmol), sodium iodide (0.15 g, 1.0 mmol), potassium carbonate (7.98 g, 57.8 mmol), 1-bromohexadecane (8.0 mL, 26 mmol), acetonitrile (250 mL); purification: column chromatography on silica gel (PE / EE 50 / 1 $\rightarrow$ 30 / 1 $\rightarrow$ 5 / 1); yield: white solid (67 %, 4.50 g, 4.63 mmol). $^{1}$H NMR (400 MHz, $CDCl_3$): $\delta$ = 0.88 (t, J = 7.1 Hz, 9H, $CH_3$), 1.23–1.48 (m, 87H, $CH_2$, $C(CH_3)_3$), 1.54–1.64 (m, 2H, $CH_2CH_2$-O-(CO)) 1.74–1.85 (m, 4H, $CH_2CH_2OAr$), 2.96–3.04 (m, 2H, $ArCH_2$), 3.90–3.98 (m, 4H, $CH_2OAr$), 4.08 (t, J = 6.7 Hz 2H, $CH_2$-O-(CO)), 4.47–4.56 (m, 1H, CHNH), 4.94 (d, J = 8.3 Hz, 1H, NH), 6.60–6.66 (m, 2H, 3-H, 5-H), 6.75–6.80 (m, 1H, 6 H) ppm; $^{13}$C NMR (126 MHz, $CDCl_3$): $\delta$ = 14.3 ($CH_3$), 22.9, 26.0, 26.2, 26.2, 28.5, 28.7, 29.4, 29.5, 29.5, 29.6, 29.6, 29.7, 29.8, 29.8, 29.9, 32.1 ($CH_2$), 38.0 ($ArCH_2$), 54.6 (CHNH), 65.7 ((CO)-$OCH_2$), 69.4, 69.4 ($ArOCH_2$), 79.9 ($C(CH_3)_3$), 114.0 (C-6), 115.1 (C-3), 121.7 (C-5), 128.66 (C-4), 148.3 (C-1), 149.2 (C-2), 155.24 (N(CO)), 172.23 ((CO)) ppm; FT-IR (ATR): $\tilde{\nu}$ = 3337 (w), 2917 (vs), 2848 (vs), 1734 (m), 1691 (vs), 1589 (w), 1532 (m), 1467 (m), 1428 (w), 1389 (w), 1367 (w), 1344 (w), 1291 (m), 1263 (s), 1169 (s), 1138 (m), 1059 (m), 849 (w), 798 (w), 722 (w), 677 (w) $cm^{-1}$; MS(EI): m/z for $C_{62}H_{115}NO_6$ calc.: 969.8724 [M], found: 970; HRMS(EI): m/z for $C_{62}H_{115}NO_6Na^+$ calc.: 969.8724 [M], found: 969.8719.

**DOPA-(12,12,12)**

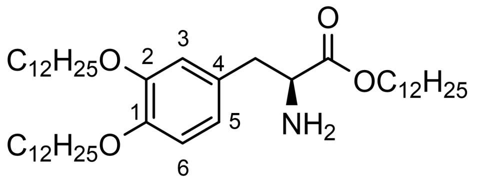


$C_{45}H_{83}NO_4$
(702.16)

Synthesis according to GP2; Boc-DOPA-(12,12,12) (0.40 g, 0.50 mmol), trifluoroacetic acid (0.40 mL, 5.2 mmol), dichloromethane (10 mL); yield: white solid (quantitive, 356 mg, 0.50 mmol); $^1$H NMR (400 MHz, $CDCl_3$): $\delta$ = 0.88 (t, J = 6.7 Hz, 9H, $CH_3$), 1.19–1.40 (m, 48H, $CH_2$), 1.40–1.51 (m, 6H, $CH_2CH_2CH_2$-O-(CO), $CH_2CH_2CH_2$-O-Ar), 1.61 (p, J = 6.9 Hz, 2H, $CH_2CH_2$-O-(CO)), 1.75–1.84 (m, 4H, $CH_2CH_2$OAr), 2.76–2.84 (m, 1H, Ar$CH_2$), 2.95–3.06 (Ar$CH_2$), 3.64 –3.72 (m, 1H, CH$NH_2$), 3.96 (t, J = 6.6 Hz, 4H, $CH_2$OAr), 4.09 (t, J = 6.8 Hz, 2H, $CH_2$-O-(CO)), 6.67–6.76 (m, 2H, 3-H, 5-H), 6.76–6.83 (m, 1H, 6-H) ppm; $^{13}$C NMR (101 MHz, $CDCl_3$): $\delta$ = 14.3 ($CH_3$), 22.8, 26.1, 26.2, 28.8, 29.4, 29.5, 29.5, 29.5, 29.6, 29.6, 29.7, 29.8, 29.8, 29.8, 29.9, 32.1 ($CH_2$), 40.9 (Ar$CH_2$), 56.1 (CH$NH_2$), 65.3 ((CO)-O$CH_2$), 69.5, 69.6 (ArO$CH_2$), 114.3 (C-6), 115.3 (C-3), 121.8 (C-5), 130.0 (C-4), 148.3 (C-1), 149.4 (C-2), 175.3 ((CO)) ppm; FT-IR (ATR): $\tilde{\nu}$=2921 (vs), 2852 (s), 1711 (m), 1512 (m), 1467(m), 1391 (w), 1366 (w), 1350 (w), 1260 (m), 1234 (m), 1166 (m), 1021 (w), 907 (s), 731 v(s), 648 (w) $cm^{-1}$; MS(ASAP): m/z for $C_{45}H_{84}NO_4^+$ calc.: 702.6395 $[M+Na]^+$, found: 703; HRMS(ASAP): m/z for $C_{45}H_{84}NO_4^+$ calc.: 702.6395 $[M+Na]^+$, found: 702.6395.

**DOPA-(16,16,16)**

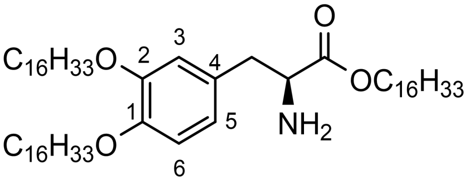


$C_{57}H_{107}NO_4$
(870.49)

Synthesis according to GP2; Boc-DOPA-(16,16,16) (0.32 g, 0.33 mmol), trifluoroacetic acid (0.25 mL, 3.3 mmol), dichloromethane (10 mL); yield: white solid (quantitive, 235 mg, 0.33 mmol); $^{1}$H NMR (400 MHz, $CDCl_3$): $\delta$ = 0.88 (t, J = 6.7 Hz, 9H, $CH_3$), 1.18–1.39 (m, 72H, $CH_2$), 1.39–1.52 (m, 6H, $CH_2CH_2CH_2$-O-(CO), $CH_2CH_2CH_2$-O-Ar) , 1.61 (p, J = 6.8 Hz, 2H, $CH_2CH_2$-O-(CO)), 1.74–1.86 (m, 4H, $CH_2CH_2$OAr), 2.75–2.84 (m, 1H, Ar$CH_2$), 2.95–3.04 (m, 1H, Ar$CH_2$), 3.68 (dd, J = 5.2 Hz, 7.7 Hz, 1H, CH$NH_2$), 3.96 (t, J = 6.6 Hz, 4H, $CH_2$OAr), 4.09 (t, J = 6.7 Hz, 2H, $CH_2$-O-(CO)), 6.66–6.74 (m, 2H, 3-H, 5-H), 6.76–6.84 (m, 1H, 6-H) ppm; $^{13}$C NMR (101 MHz, $CDCl_3$): $\delta$ = 14.3 ($CH_3$), 22.9, 26.1, 26.2, 28.8, 29.4, 29.5, 29.5, 29.6, 29.7, 29.8, 29.8, 29.9, 32.1 ($CH_2$), 40.9 (Ar$CH_2$), 56.1 (CH$NH_2$), 65.3 ((CO)-O$CH_2$), 69.5, 69.6 (ArO$CH_2$) 114.3 (C-6), 115.3 (C-3), 121.8 (C-5), 130.0 (C-4), 148.3 (C-1), 149.4 (C-2), 175.3 ((CO)) ppm; FT-IR (ATR): $\tilde{\nu}$ = 2956 (m), 2917 (vs), 2850 (vs), 1736 (w), 1677 (w), 1591 (w), 1516 (m), 1467(m), 1430 (w), 1379 (w), 1265 (m), 1236 (m), 1201 (m), 1138 (m), 1018 (w), 908 (m), 800 (w), 734 (s) $cm^{-1}$; MS(ESI): m/z for $C_{57}H_{108}NO_4^+$ calc.: 870.8273 $[M+H]^+$, found: 871; HRMS(ESI): m/z for $C_{57}H_{108}NO_4^+$ calc.: 870.8273 $[M+H]^+$, found: 870.8273.

**Cy12**

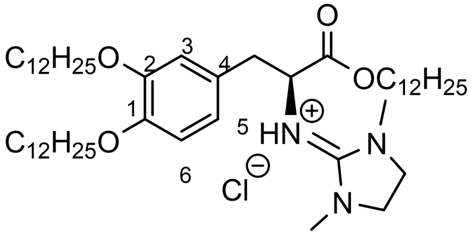

$C_{50}H_{92}ClN_3O_4$
834.75 g/mol

Synthesis according to GP3; DOPA-(12,12,12) (2.00 g, 2.85 mmol), $NaHCO_3$ (2.39 g, 28.5 mmol), 2-chloro-1,3-dimethyl-4,5-dihydro-1H-imidazol-3-ium chloride (3.7 mL, 1 M, 3.7 mmol), dichloromethane (30 mL); purification: column chromatography on silica gel (dichloromethane/ methanol 15/1); yield: colorless solid (51%, 1.20 g, 1.44 mmol); melting behavior: Cr 39 °C (–23.4 kJ/mol) Colh 62 °C (–0.3 kJ/mol) I 62 °C (0.7 kJ/mol) $Col_h$ 32 °C (17.4 kJ/mol) Cr; $^1$H NMR (500 MHz, $CDCl_3$): $\delta$ = 0.86 (t, J = 6.8 Hz, 9H, $CH_3$), 1.20–1.36 (m, 50H, $CH_2$), 1.39–1.48 (m, 4H, $CH_2CH_2CH_2$-O-Ar), 1.61–1.69 (m, 2H, $CH_2CH_2$-O-(CO)), 1.72–1.80 (m, 4H, $CH_2CH_2OAr$), 2.98 (s, 6H, $NCH_3$), 3.23–3.30 (m, 1H, $ArCH_2$), 3.41–3.48 (m, 2H, $NCH_2$); 3.60–3.68 (m, 2H, $NCH_2$), 3.67–3.77 (m, 1H, $ArCH_2$), 3.89–4.20 (m, 7H, CHNH, $CH_2$-O-(CO), $CH_2OAr$), 6.78 (d, J = 8.1 Hz, 1H, 3-H), 7.02 (dd, J = 1.9 Hz, 8.2 Hz, 1H, 5-H), 7.13 (s, 1H, 6-H), 9.86 (s, 1H, NH) ppm; $^{13}$C NMR (126 MHz, $CDCl_3$): $\delta$ = 14.1 ($CH_3$), 22.7, 25.9, 26.1, 26.1, 28.5, 29.3, 29.4, 29.4, 29.4, 29.4, 29.5, 29.6, 29.6, 29.7, 29.7, 29.7, 29.7, 31.9, 31.9 ($CH_2$), 36.1, ($NCH_3$), 36.4 ($ArCH_2$) 49.3 ($NCH_2$), 60.8 (CHN), 66.5 ((CO)-$OCH_2$), 69.5, 69.6, ($ArOCH_2$), 114.1 (C-3), 116.0 (C-6), 122.2 (C-5), 130.1 (C-4), 148.1 (C-1), 149.1 (C-2), 161.3 (NCN), 170.6 ((CO)) ppm; FT-IR (ATR): $\tilde{\nu}$ = 2921 (vs), 2852 (vs), 2171 (w), 1739 (m), 1628 (s), 1511 (s), 1467 (s), 1429 (m), 1379 (m), 1261 (s), 1233 (m), 1139 (m), 1034 (m), 927 (m), 802 (w), 726 (vs), 639 (w) $cm^{-1}$; MS(ESI): m/z for $C_{50}H_{92}N_3O_4^+$ calc.: 798.7082 $[M-Cl]^+$, found: 799; HRMS(ESI): m/z for $C_{50}H_{92}N_3O_4^+$ calc.: 798.7082 $[M-Cl]^+$, found: 798.7082.

**Cy14**

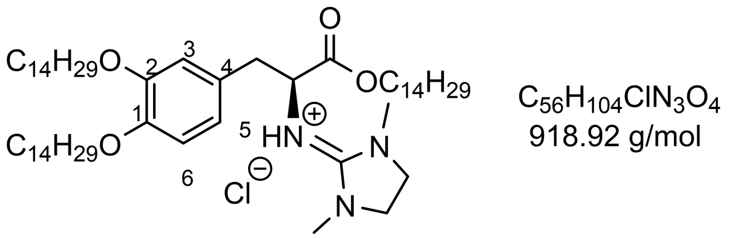


Synthesis according to GP3; DOPA-(14,14,14) (5.00 g, 6.36 mmol), $NaHCO_3$ (5.34 g, 63.6 mmol), 2-chloro-1,3-dimethyl-4,5-dihydro-1H-imidazol-3-ium chloride (9.5 mL, 1 M, 9.5 mmol), dichloromethane (40 mL); purification: column chromatography on silica gel (dichloromethane/ methanol 15/1); yield: colorless solid (38%, 2.215 g, 2.41 mmol); melting behavior: Cr 54 °C (–36.5 kJ/mol) I 57 °C (0.4 kJ/mol) $Col_h$ 50 °C (33.2 kJ/mol) Cr; $^1$H NMR (500 MHz, $CDCl_3$): $\delta$ = 0.86 (t, J = 6.9 Hz, 9H, $CH_3$), 1.17–1.38 (m, 62H, $CH_2$), 1.38–1.48 (m, 4H, $CH_2CH_2CH_2$-O-Ar), 1.60–1.69 (m, 2H, $CH_2CH_2$-O-(CO)), 1.72–1.81 (m, 4H, $CH_2CH_2OAr$), 2.98 (s, 6H, $NCH_3$), 3.19–3.31 (m, 1H, $ArCH_2$), 3.40–3.51 (m, 2H, $NCH_2$); 3.60–3.67 (m, 2H, $NCH_2$), 3.68–3.77 (m, 1H, $ArCH_2$), 3.88–4.20 (m, 7H, CHNH, $CH_2$-O-(CO), $CH_2OAr$), 6.78 (d, J = 8.2 Hz, 1H, 3-H), 7.02 (dd, J = 2.0 Hz, 8.1 Hz, 1H, 5-H), 7.13 (s, 1H, 6-H), 9.87 (d, J = 9.3 Hz, 1H, NH) ppm; $^{13}$C NMR (126 MHz, $CDCl_3$): $\delta$ = 14.1 ($CH_3$), 22.7, 25.9, 26.1, 28.5, 29.3, 29.4, 29.4, 29.4, 29.5, 29.6, 29.6, 29.7, 29.7, 29.7, 29.7, 29.7, 31.9 ($CH_2$), 36.1 ($NCH_3$), 36.4 ($ArCH_2$), 49.3 ($NCH_2$), 60.8 (CHN), 66.5 ((CO)-$OCH_2$), 69.5, 69.6, ($ArOCH_2$), 114.1 (C-3), 116.0 (C-6), 122.2 (C-5), 130.1 (C-4), 148.1 (C-1), 149.1 (C-2), 161.4 (NCN), 170.6 ((CO)) ppm FT-IR (ATR): $\tilde{\nu}$ = 2922 (s), 2853 (m), 2184 (w), 1742 (m), 1631 (m), 1511 (m), 1467 (m), 1428 (w), 1379 (w), 1262 (m), 1234 (m), 1139 (w), 1034 (w), 984 (w), 924 (m), 908 (s), 727 (vs), 640 (m) $cm^{-1}$; MS(ESI): m/z for $C_{56}H_{104}N_3O_4^+$ calc.: 882.8021 $[M-Cl]^+$, found: 883; HRMS(ESI): m/z for $C_{56}H_{104}N_3O_4^+$ calc.: 882.8021 $[M-Cl]^+$, found: 882.8021.

**Cy16**

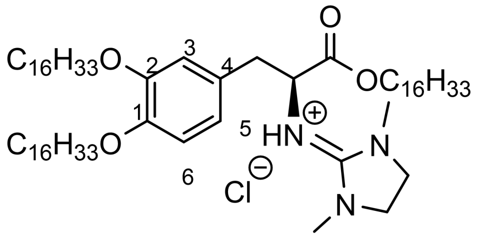


$C_{62}H_{116}ClN_3O_4$
1003.08 g/mol

Synthesis according to GP3; DOPA-(16,16,16) (5.45 g, 6.26 mmol), $NaHCO_3$ (5.26 g, 62.6 mmol), 2-chloro-1,3-dimethyl-4,5-dihydro-1H-imidazol-3-ium chloride (9.4 mL, 9.4 mmol), dichloromethane (40 mL); purification: column chromatography on silica gel (dichloromethane/ methanol 15/1); yield: colorless solid (36$, 2.27 g, 2.27 mmol); melting behavior: Cr 63 °C (–56.0 kJ/mol) $Col_h$ 104 °C (–1.4 kJ/mol) I 106 °C (1.5 kJ/mol) Colh 60 °C (52.7 kJ/mol) Cr; $^1$H NMR (500 MHz, $CDCl_3$): $\delta$ = 0.81 (t, J = 6.9 Hz, 9H, $CH_3$), 1.14–1.32 (m, 74H, $CH_2$), 1.34–1.43 (m, 4H, $CH_2CH_2CH_2$-O-Ar), 1.57–1.64 (m, 2H, $CH_2CH_2$-O-(CO)), 1.67–1.76 (m, 4H, $CH_2CH_2OAr$), 2.93 (s, 6H, $NCH_3$), 3.19–3.25 (m, 1H, $ArCH_2$), 3.40 (d, J = 9.4 Hz 2H, $NCH_2$); 3.60 (d, J = 11.7 Hz 2H, $NCH_2$), 3.64–3.72 (m, 1H, $ArCH_2$), 3.84–4.16 (m, 7H, CHNH, $CH_2$-O-(CO), $CH_2OAr$), 6.73 (d, J = 8.0 Hz, 1H, 3-H), 6.97 (d, J = 8.0 Hz, 1H, 5-H), 7.08 (s, 1H, 6-H), 9.86 (s, 1H, NH) ppm; $^{13}$C NMR (126 MHz, $CDCl_3$): $\delta$ = 14.1 ($CH_3$), 22.7, 25.9, 26.1, 26.2, 28.5, 29.3, 29.4, 29.4, 29.5, 29.5, 29.6, 29.6, 29.7, 29.7, 29.7, 29.8, 31.9 ($CH_2$), 36.1, ($NCH_3$), 36.4 ($ArCH_2$) 49.3 ($NCH_2$), 60.8 (CHN), 66.5 ((CO)-$OCH_2$), 69.5, 69.6, ($ArOCH_2$), 114.1 (C-3), 116.0 (C-6), 122.2 (C-5), 130.1 (C-4), 148.1 (C-1), 149.2 (C-2), 161.4 (NCN), 170.6 ((CO)) ppm; FT-IR (ATR): $\tilde{\nu}$ = 2921 (s), 2852 (s), 2195 (w), 1742 (w), 1632 (w), 1591 (m), 1511 (w), 1467 (m), 1429 (w), 1379 (w), 1262 (m), 1139 (w), 1035 (w), 907 (s), 727 (vs), 641 (m) $cm^{-1}$; MS(ESI): m/z for $C_{62}H_{116}N_3O_4^+$ calc.: 966.8960 $[M-Cl]^+$, found: 967; HRMS(ESI): m/z for $C_{62}H_{116}N_3O_4^+$ calc.: 966.8960 $[M-Cl]^+$, found: 966.8960.

**Ac12**

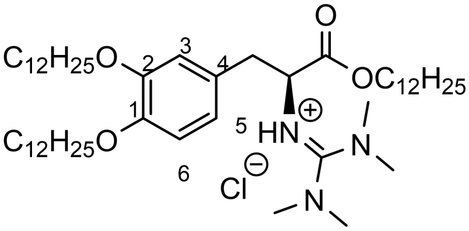


$C_{50}H_{94}ClN_3O_4$
836.77 g/mol

Synthesis according to GP3; DOPA-(12,12,12) (2.00 g, 2.84 mmol), $NaHCO_3$ (2.35 g, 28.0 mmol), tetramethylguanidinium chloride (3.13 mL, 3.13 mmol), dichloromethane (30 mL); purification: column chromatography on silica gel (dichloromethane/methanol 15/1); yield: colorless solid (51%, 1.205 g, 1.44 mmol); melting behavior: Cr 66 °C (–31.3 kJ/mol) I 53 °C (1.2 kJ/mol) Colh 30 °C (15.0 kJ/mol) Cr; $^1H$ NMR (500 MHz, $CDCl_3$): $\delta$ = 0.86 (t, J = 6.9 Hz, 9H, $CH_3$), 1.09–1.50 (m, 54H, $CH_2$), 1.56 (t, J = 6.9 Hz, 2H, $CH_2CH_2$-O-(CO)), 1.72–1.86 (m, 4H, $CH_2CH_2OAr$), 2.35–3.61 (m, 12H, $NCH_3$), 3.23–3.30 (1H, m, $ArCH_2$), 3.64–3.74 (m, 1H, $ArCH_2$), 3.88–4.13 (m, 7H, CHNH, $CH_2OAr$, $CH_2$-O-(CO)), 6.77 (d, J = 8.2 Hz, 1H, 3-H), 6.97 (d, J = 8.1 Hz, 1H, 5-H), 7.07 (s, 1H, 6-H), 10.02–10.09 (m, 1H, NH) ppm; $^{13}C$ NMR (126 MHz, $CDCl_3$): $\delta$ = 14.2 ($CH_3$), 22.7, 22.8, 26.1, 26.1, 28.4, 29.2, 29.4, 29.4, 29.4, 29.5, 29.5, 29.5, 29.6, 29.7, 29.7, 29.7, 29.7, 31.9, 31.9 ($CH_2$), 36.4 ($NCH_3$), 39.6 ($ArCH_2$), 60.6 (CHN), 66.3 ((CO)-$OCH_2$), 69.4, 69.5, ($ArOCH_2$), 114.0 (C-3), 115.7 (C-6), 122.1 (C-5), 129.4 (C-4), 148.1 (C-1), 149.1 (C-2), 162.17 (NCN), 175.3 ((CO)) ppm; FT-IR (ATR): $\tilde{\nu}$ = 3386 (w), 2956 (m), 2912 (vs), 2851 (vs), 1735 (m), 1626 (m), 1572 (m), 1516 (m), 1468 (m), 1431 (m), 1405 (m), 1265 (m), 1234 (m), 1172 (m), 1142 (m), 1029 (w), 721 (w) $cm^{-1}$; MS(ESI): m/z for $C_{50}H_{94}N_3O_4^+$ calc.: 800.7239 $[M-Cl]^+$, found: 801; HRMS(ESI): m/z for $C_{50}H_{94}N_3O_4^+$ calc.: 800.7239 $[M-Cl]^+$, found: 800.7239.

**Ac16**

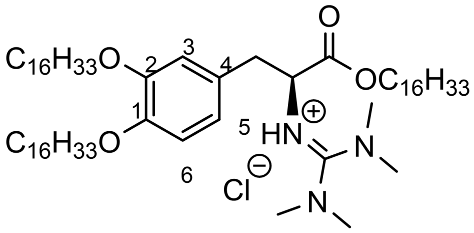


$C_{62}H_{118}ClN_3O_4$
1005.88 g/mol

Synthesis according to GP3; DOPA-(16,16,16) (2.00 g, 2.30 mmol), $NaHCO_3$ (1.93 g, 23.0 mol), tetramethylguanidinium chloride (2.53 mL, 1 M, 2.53 mmol), dichloromethane (30 mL); purification: column chromatography on silica gel (dichloromethane/methanol 15/1); yield: colorless solid (9%, 180 mg, 0.18 mmol); melting behavior: Cr 65 °C (–73.7 kJ/mol) Colh 98 °C (–1.4 kJ/mol) I 100 °C (1.6 kJ/mol) Colh 63 °C (76.7 kJ/mol) Cr; $^1$H NMR (500 MHz, $CDCl_3$): $\delta$ = 0.81 (t, J = 6.9 Hz, 9H, $CH_3$), 1.13–1.33 (m, 74H, $CH_2$), 1.34–1.42 (m, 4H, $CH_2CH_2CH_2$-O-Ar), 1.51 (p, J = 6.8 Hz, 2H, $CH_2CH_2$-O-(CO)), 1.67–1.76 (m, 4H, $CH_2CH_2OAr$), 2.42–3.51 (m, 12H, $NCH_3$), 3.19–3.24 (1H, m, $ArCH_2$), 3.59–3.69 (m, 1H, $ArCH_2$), 3.82–3.93 (m, 3H, CHNH, $CH_2$-O-(CO)), 3.94–4.06(m, 4H, $CH_2OAr$), 6.72 (d, J = 8.0 Hz, 1H, 3-H), 6.91 (d, J = 8.0 Hz, 1H, 5-H), 7.02 (s, 1H, 6-H), 9.98 (s, 1H, NH) ppm; $^{13}$C NMR (126 MHz, $CDCl_3$): $\delta$ = 14.1 ($CH_3$), 22.7, 25.9, 26.1, 26.2, 28.5, 29.2, 29.4, 29.4, 29.5, 29.6, 29.6, 29.6, 29.7, 29.7, 29.7, 29.7, 29.8, 32.0 ($CH_2$), 36.4 ($NCH_3$), 39.6 ($ArCH_2$), 60.6 (CHN), 66.3 ((CO)-$OCH_2$), 69.4, 69.6, ($ArOCH_2$), 114.0 (C-3), 115.8 (C-6), 122.2 (C-5), 129.4 (C-4), 148.1 (C-1), 149.1 (C-2), 162.18 (NCN), 171.1 ((CO)) ppm; FT-IR (ATR): $\tilde{\nu}$ = 2917 (vs), 2850 (s), 2187 (w), 1737 (m), 1624 (m), 1572 (m), 1514 (m), 1467 (m), 1431 (w), 1405 (w), 1265 (m), 1234 (m), 1169 (w), 1029 (w), 926 (m), 909 (m), 730 (s), 641 (w) cm$^{-1}$; MS(ESI): m/z for $C_{62}H_{118}N_3O_4^+$ calc.: 968.9117 [M-Cl]$^+$, found: 969; HRMS(ESI): m/z for $C_{62}H_{118}N_3O_4^+$ calc.: 968.9117 [M-Cl]$^+$, found: 968.9117.

# NMR Spectra

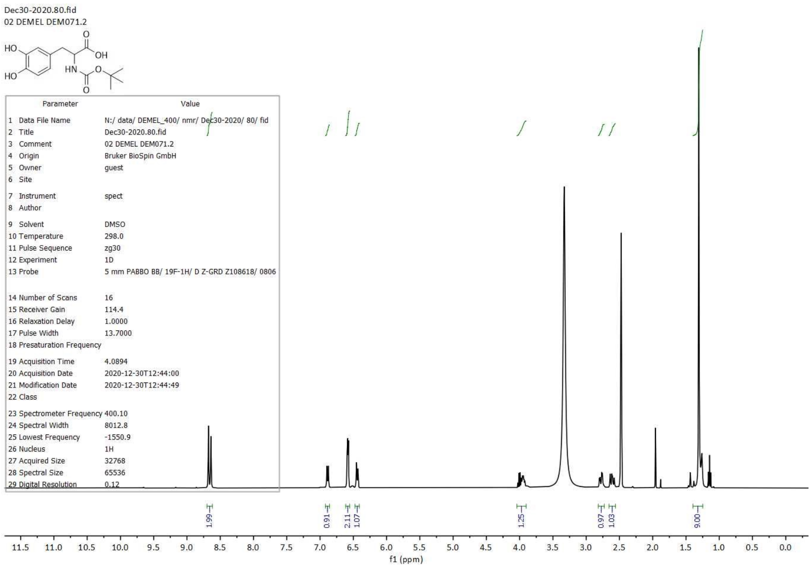


Fig. S1: $^{1}$H NMR spectrum of Boc-DOPA in DMSO-d6 at 400 MHz

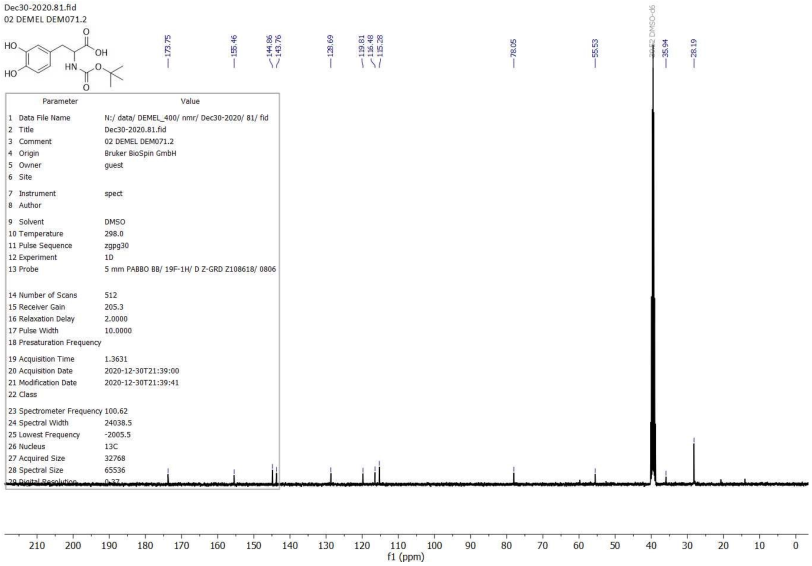


Fig. S2: $^{13}$C NMR spectrum of Boc-DOPA in DMSO-d6 at 101 MHz

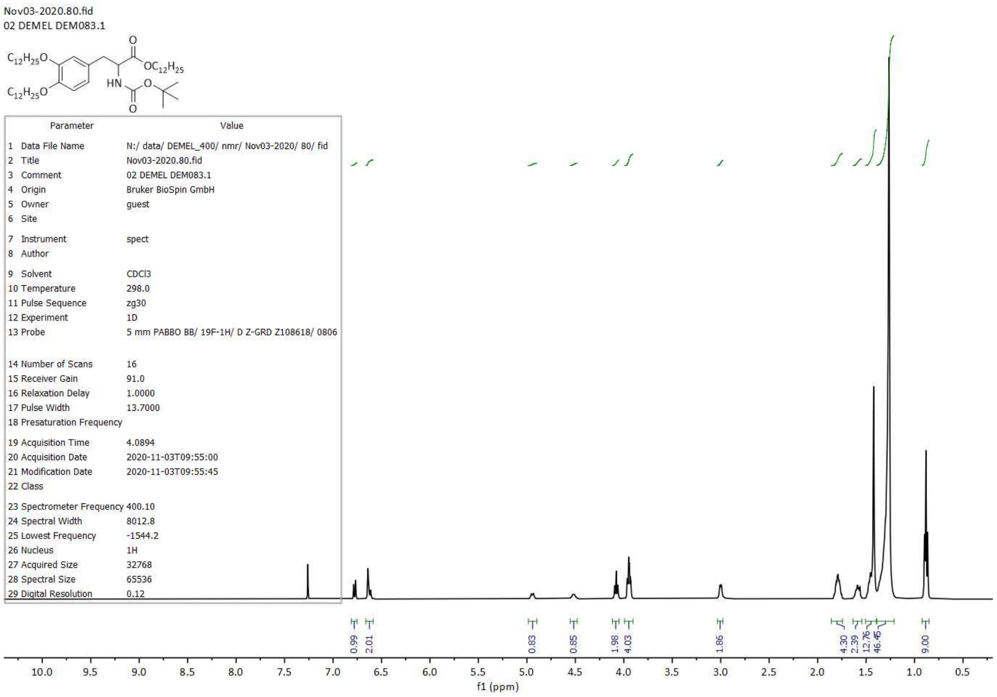


Fig. S3: $^{1}H$ NMR spectrum of Boc-DOPA-(12,12,12) in $CDCl_3$ at 400 MHz

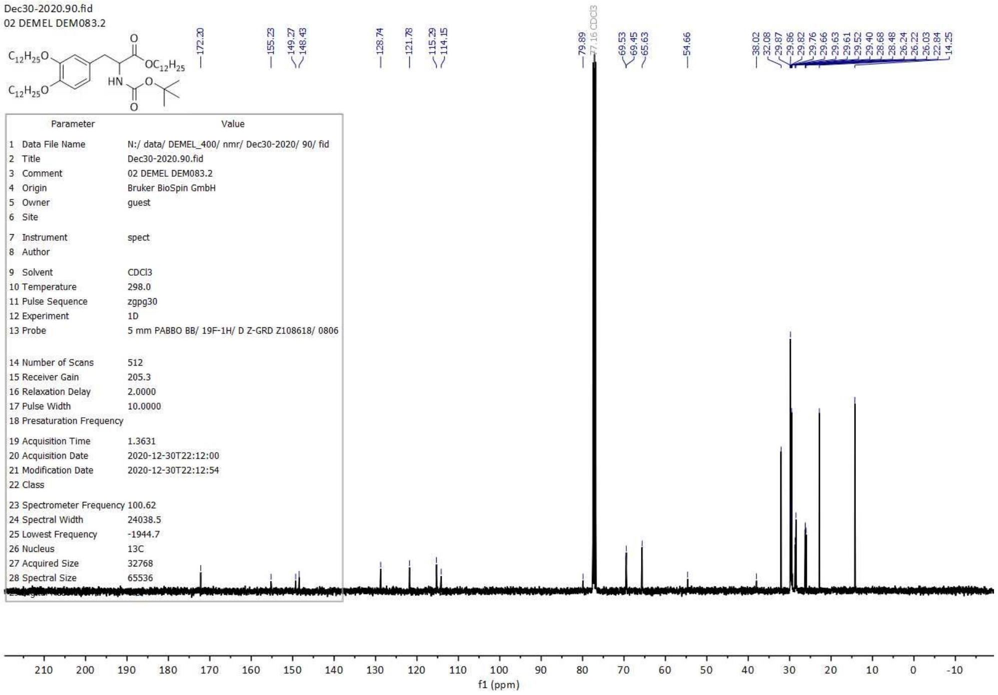


Fig. S4: $^{13}C$ NMR spectrum of Boc-DOPA-(12,12,12) in $CDCl_3$ at 101 MHz

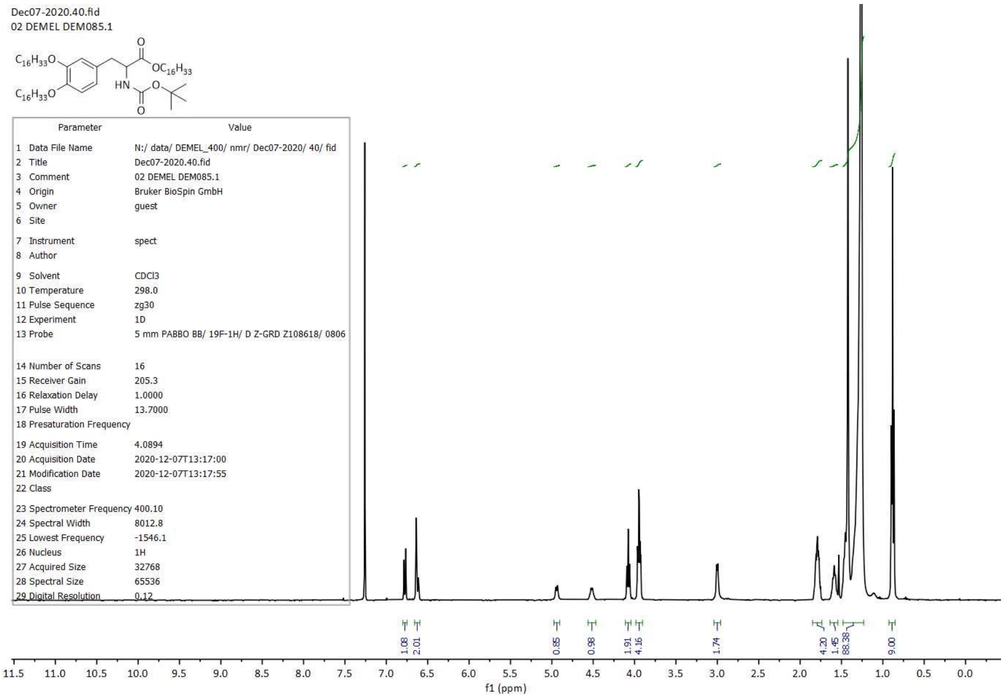


Fig. S5: $^{1}$H NMR spectrum of Boc-DOPA-(16,16,16) in $CDCl_3$ at 400 MHz

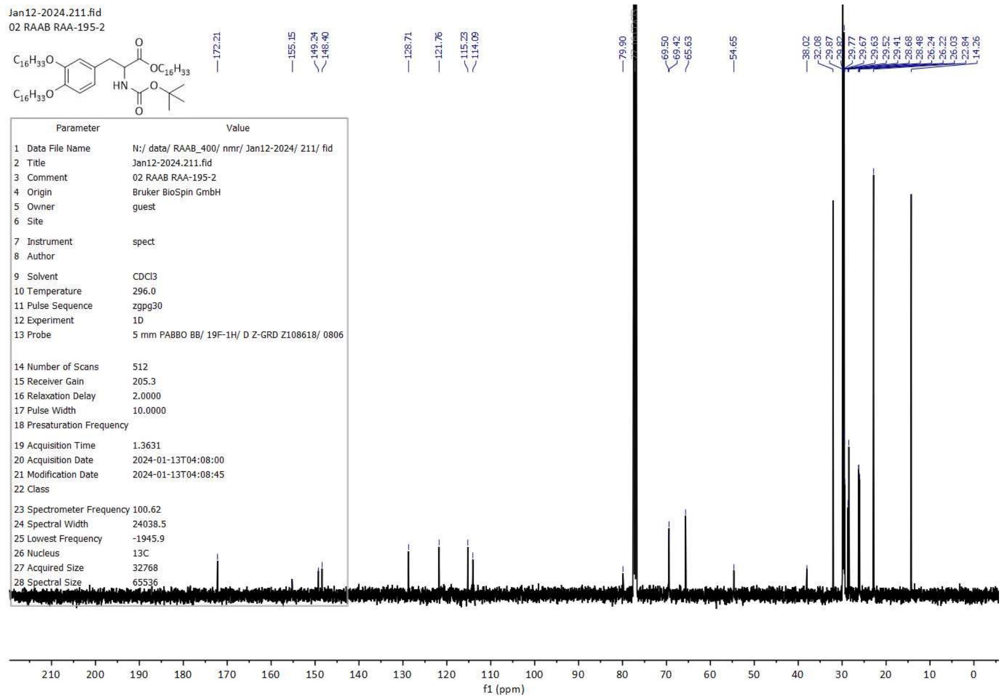


Fig. S6: $^{13}$C NMR spectrum of Boc-DOPA-(16,16,16) in $CDCl_3$ at 101 MHz

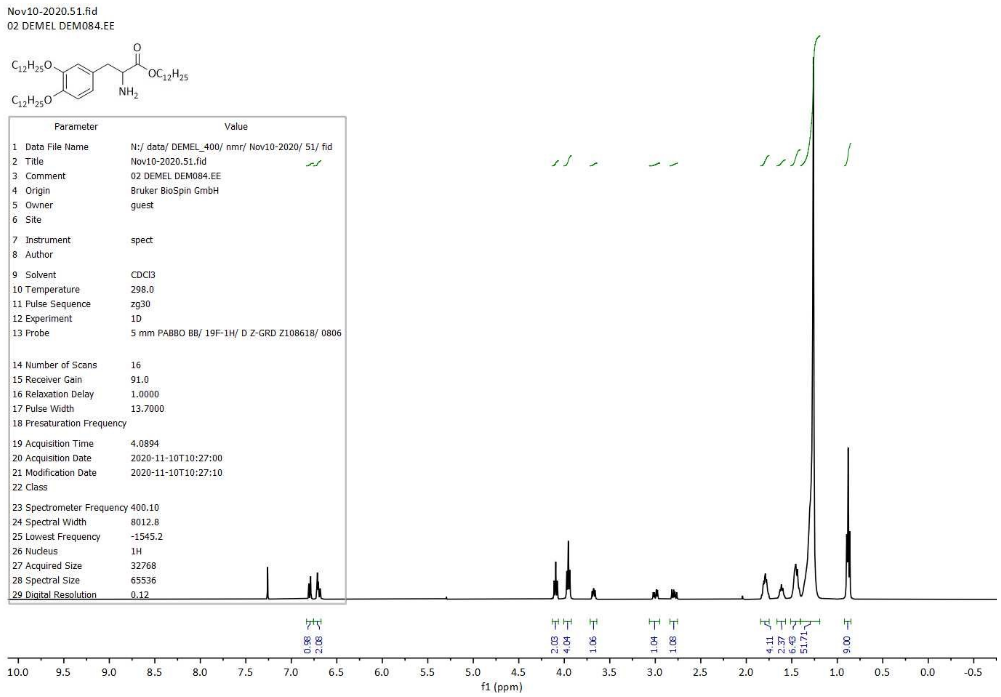

Fig. S7: $^{1}H$ NMR spectrum of DOPA-(12,12,12) in $CDCl_3$ at 400 MHz

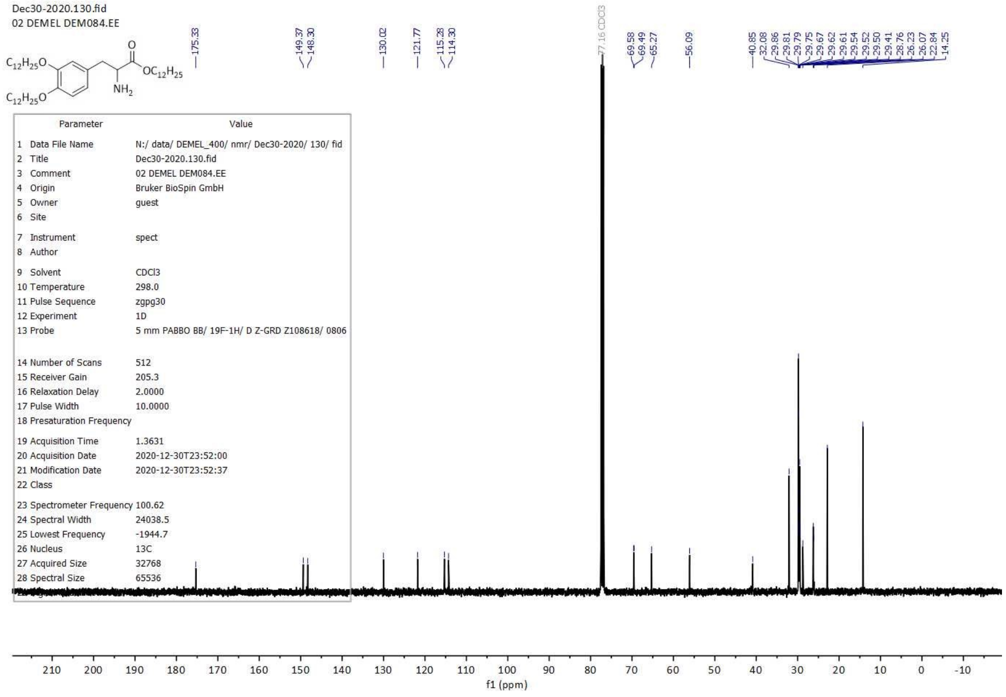

Fig. S8: $^{13}C$ NMR spectrum of DOPA-(12,12,12) in $CDCl_3$ at 101 MHz

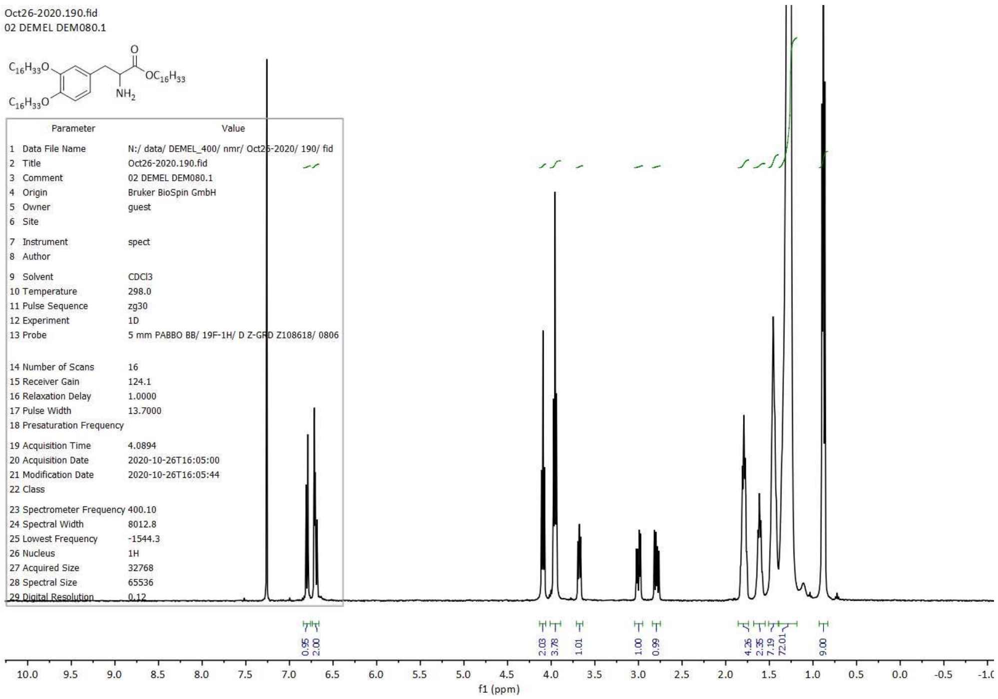

Fig. S9: $^{1}H$ NMR spectrum of DOPA-(16,16,16) in $CDCl_3$ at 400 MHz

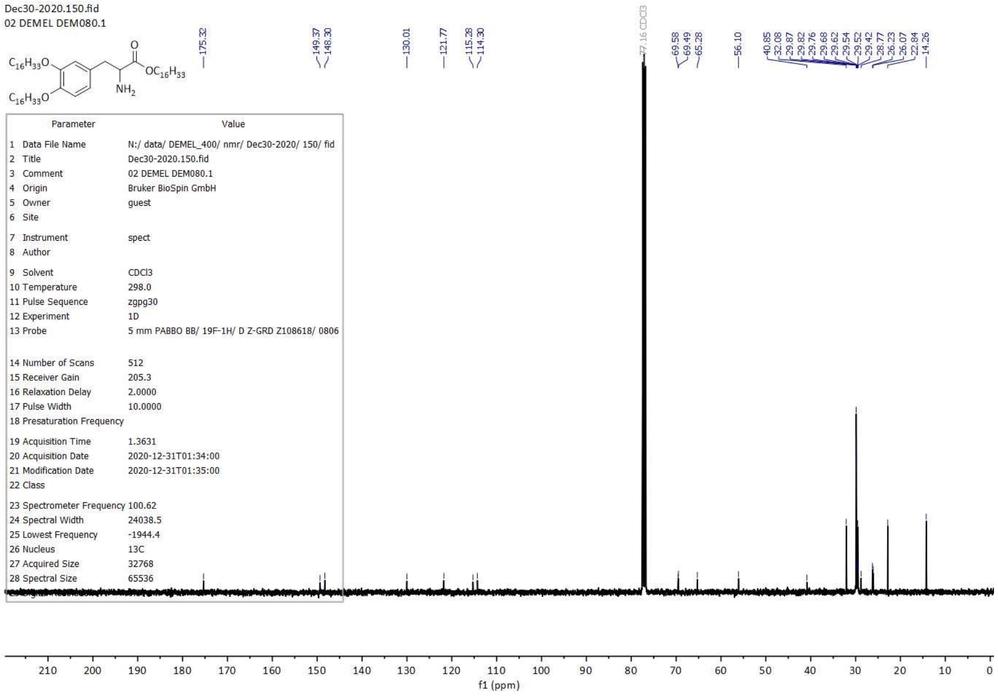

Fig. S10: $^{13}C$ NMR spectrum of DOPA-(16,16,16) in $CDCl_3$ at 101 MHz

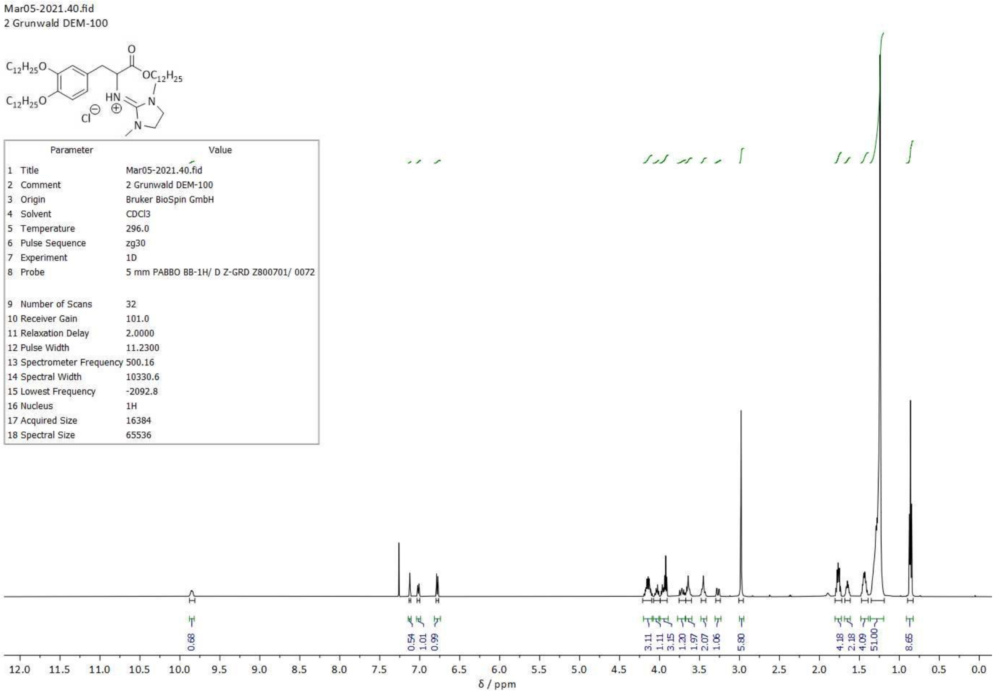


Fig. S11: $^{1}$H NMR spectrum of Cy12 in $CDCl_3$ at 500 MHz

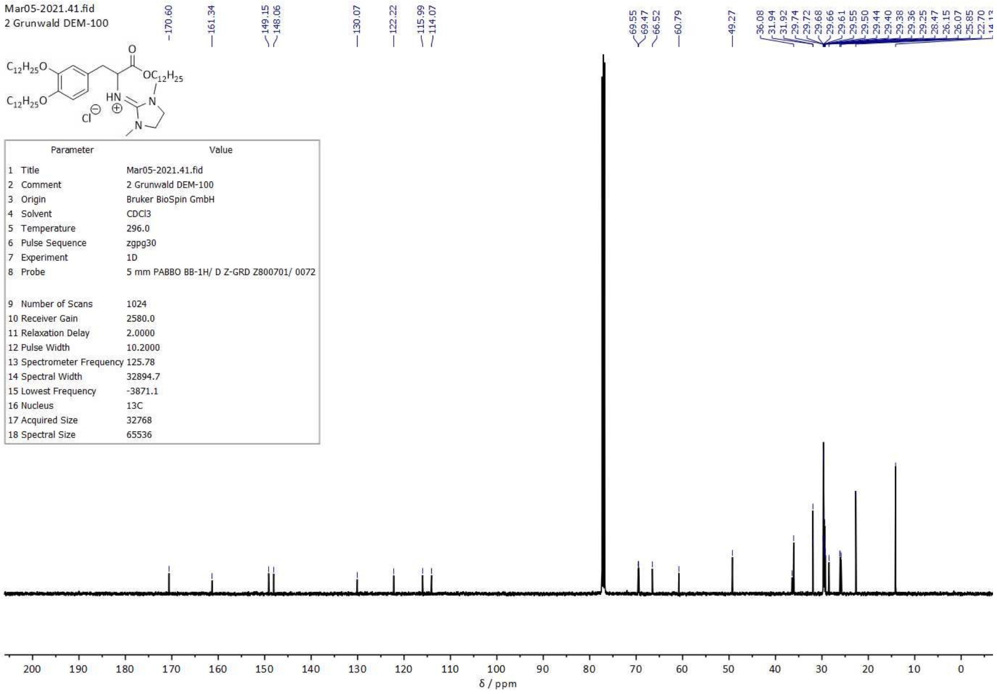


Fig. S12: $^{13}$C NMR spectrum of Cy12 in $CDCl_3$ at 126 MHz

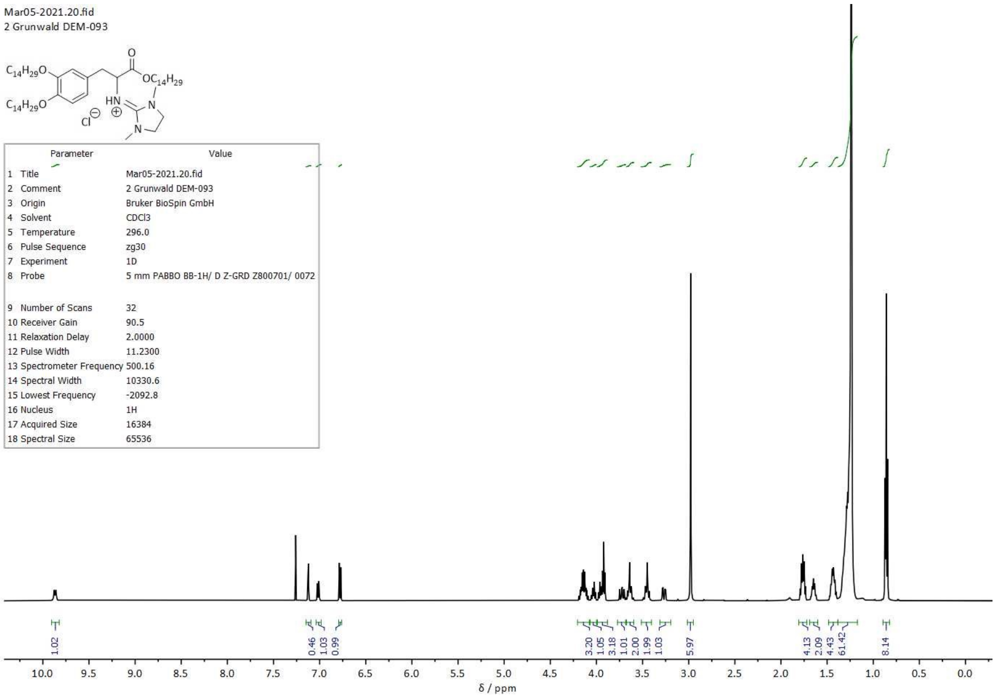


Fig. S13: $^{1}$H NMR spectrum of Cy14 in $CDCl_3$ at 500 MHz

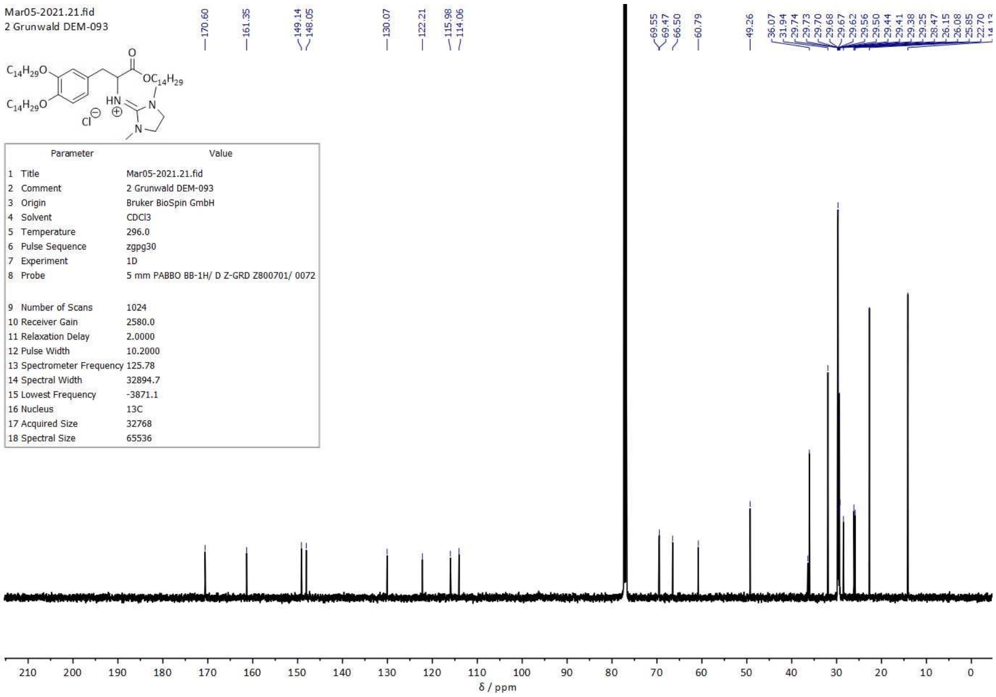


Fig. S14: $^{13}$C NMR spectrum of Cy14 in $CDCl_3$ at 101 MHz

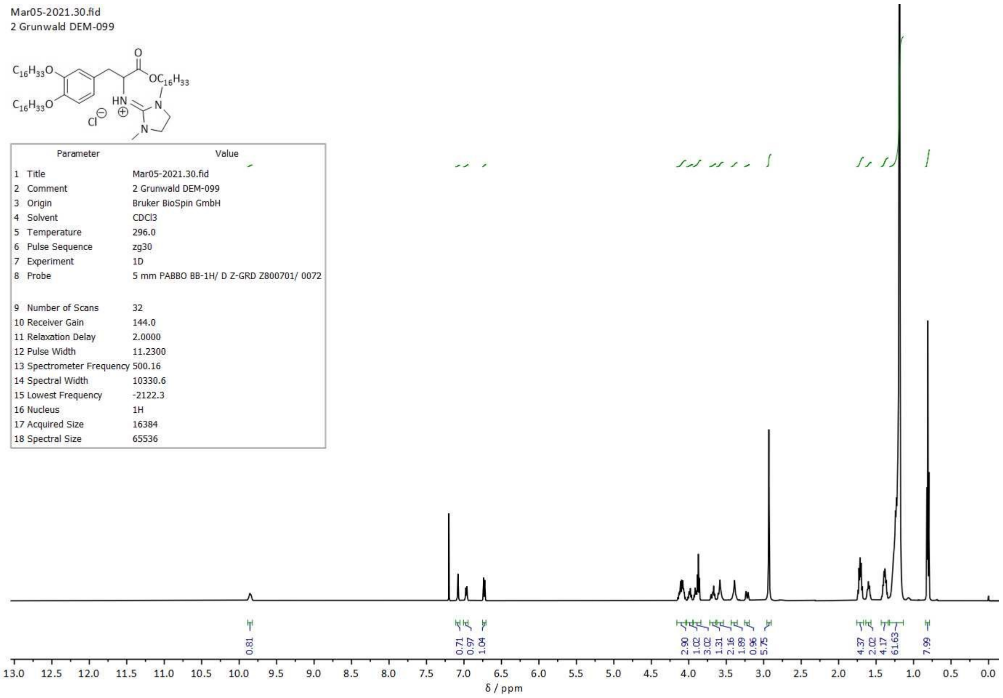


Fig. S15: $^{1}H$ NMR spectrum of Cy16 in $CDCl_3$ at 500 MHz

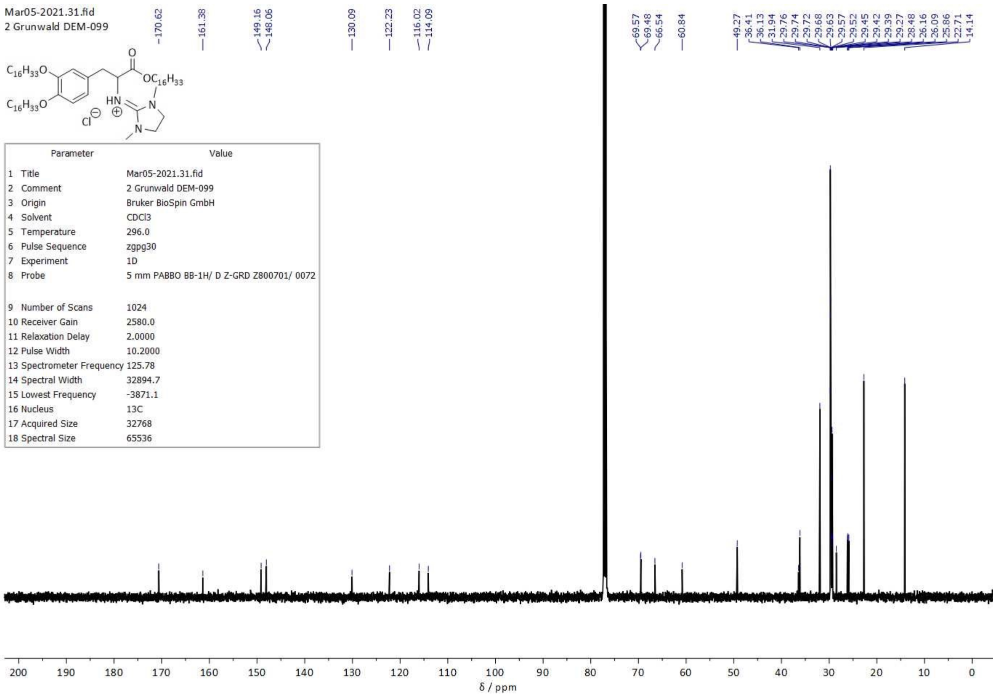


Fig. S16: $^{13}C$ NMR spectrum of Cy16 in $CDCl_3$ at 101 MHz

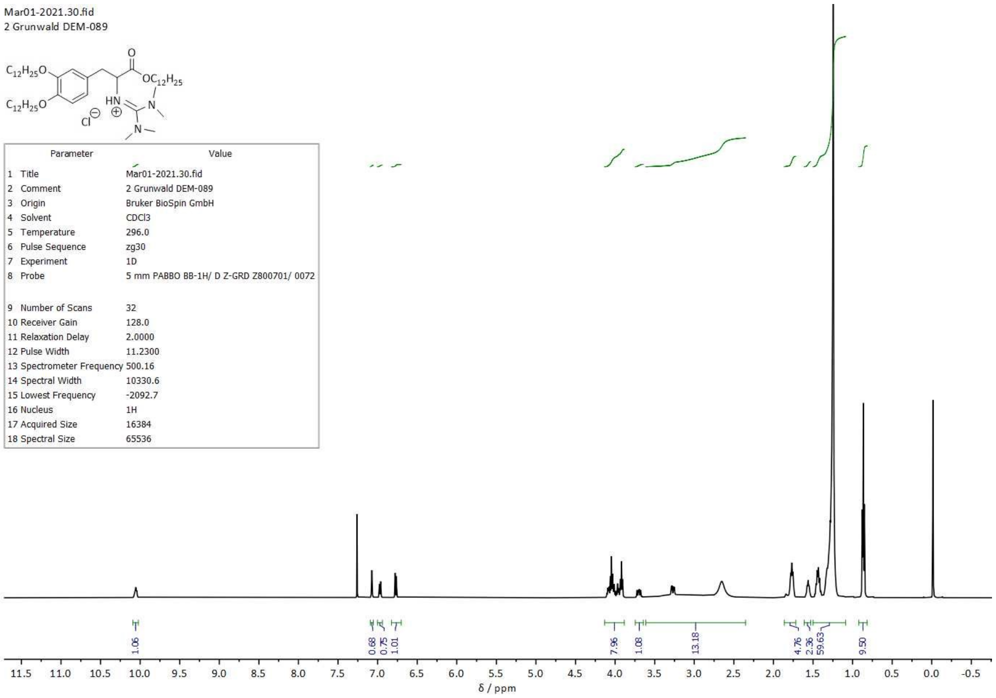


Fig. S17: $^{1}$H NMR spectrum of Ac12 in $CDCl_3$ at 500 MHz

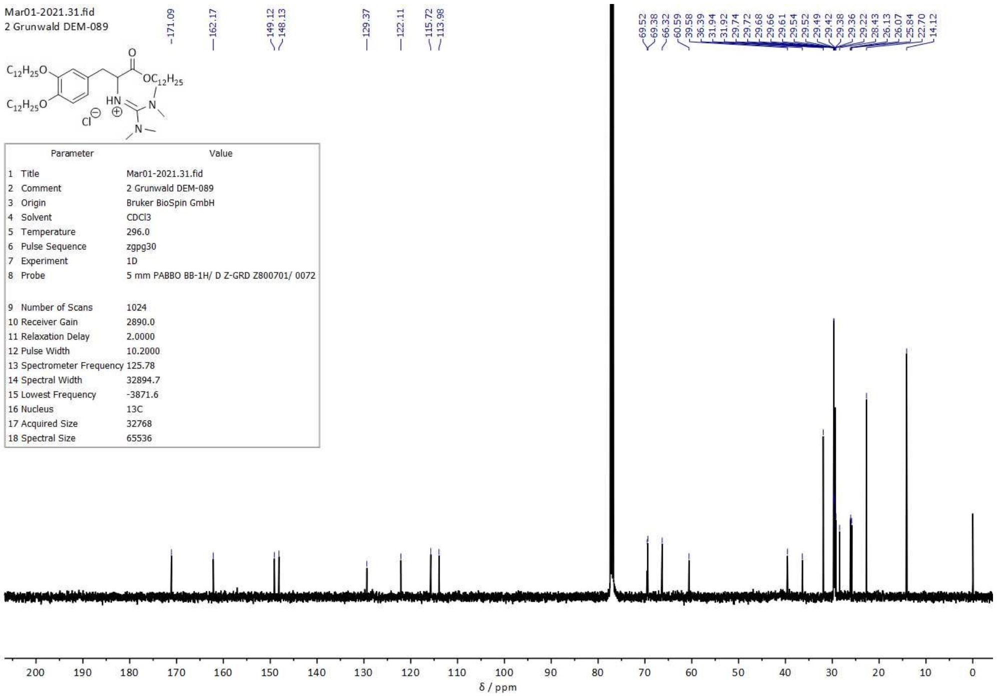


Fig. S18: $^{13}$C NMR spectrum of Ac12 in $CDCl_3$ at 126 MHz

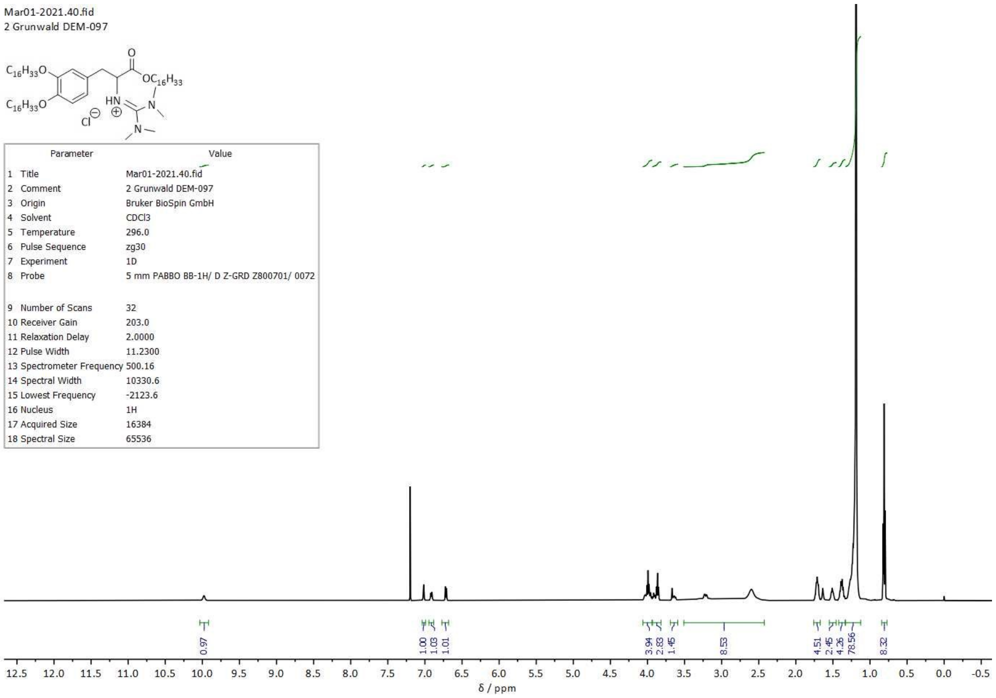

Fig. S19: $^{1}$H NMR spectrum of Ac16 in $CDCl_3$ at 500 MHz

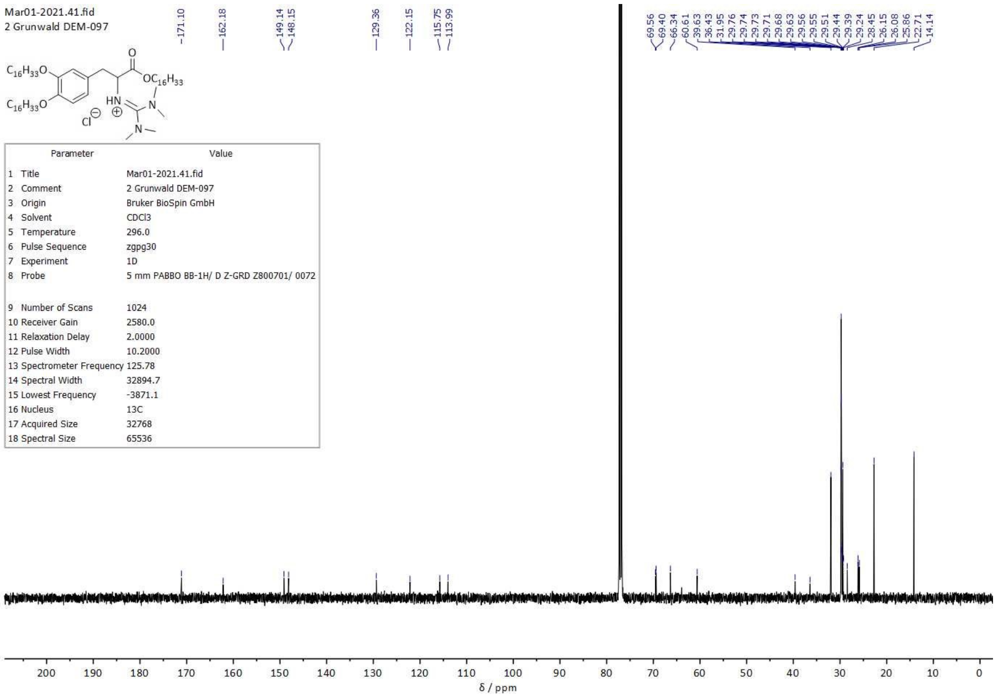

Fig. S20: $^{13}$C NMR spectrum of Ac16 in $CDCl_3$ at 126 MHz

# Optical Birefringence Measurement

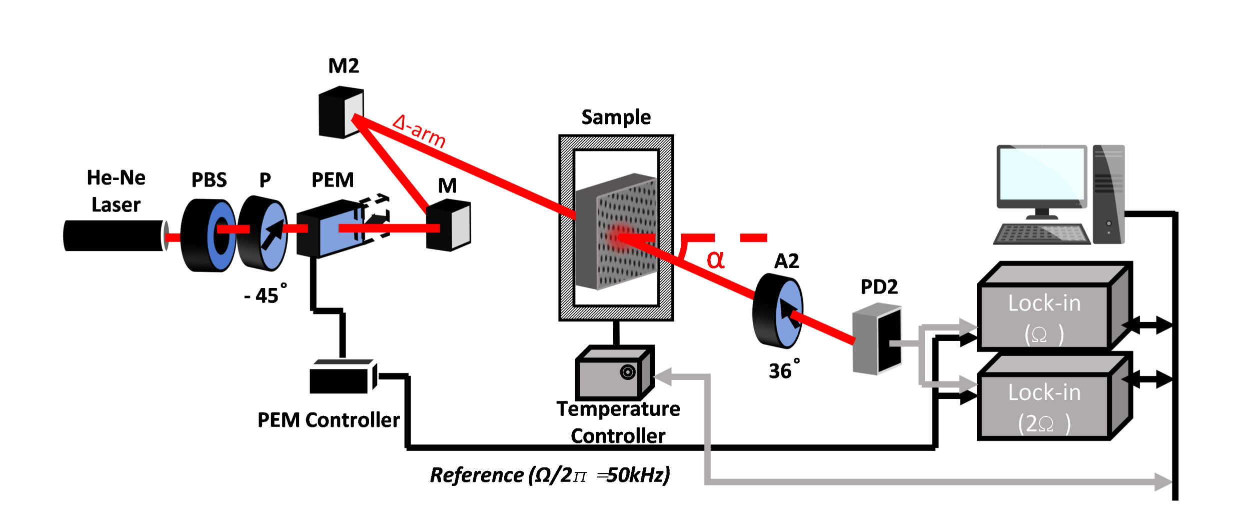


Fig. S21: **Sketch of the setup for birefringence measurements.** PBS is the polarising beam splitter, which splits the laser beam into a Ψ arm and a Δ arm. For birefringence measurement in this work only the Δ arm is used. P refers to the polariser. PEM is the Photon Elastic Modulator. M1 and M2 are the mirrors and $\lambda/4$ is a quarter wave plate. The sample is placed in a sealed sample chamber with an argon atmosphere. A2 is the analyser with its polarisation direction perpendicular to the polariser. PD2 is the photodiode that detects the modularised light and transfers the data to the corresponding lock-in amplifier for further analysis.

A He-Ne laser ($\lambda = 632.8$ nm) is used as a linearly polarised light source. The laser beam first passes through a polariser in order to be linearly polarised at an angle of 45 degrees to the direction of propagation. The photoelastic modulator (PEM) is used to apply a time-modulated delay to the beam. The beam measuring the linear birefringence ($\delta$ -arm) is reflected by two mirrors and passes through the sample at an angle of incidence of $\alpha = 36°$. The beam then passes through an analyser set perpendicular to the polariser and reach the photodiode. Two SR830 lock-in amplifiers from Stanford Research Systems (Sunnyvale, USA) connected to the detector measure the amplitudes of the 1st and 2nd harmonics using two reference signals that are locked at 50 and 100 kHz from the modulated light intensities. The corresponding optical retardation is calculated from the measured light intensities.

To measure the optical birefringence of bulk Dopa-ILCs, the materials are infiltrated into slit cells with a well-defined 10 µm spacing and polymer-coated hydrophobic surfaces. In contrast to

the confined samples, the three cyclic Dopa-ILCs all show a sharp change in order parameters at the phase transition temperature, which is characteristic of first order phase transitions.

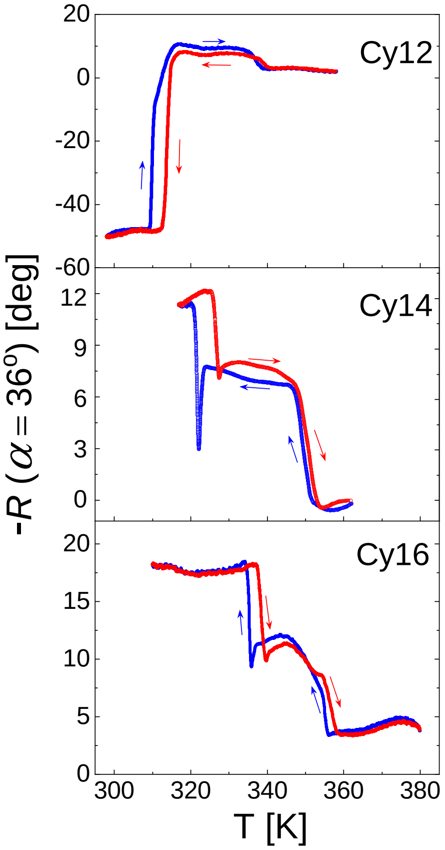


Fig. S22: **Optical retardation curves of bulk cyclic Dopa-ILCs of different side chain lengths (n = 12, 14 and 16).** The measurements record the 2nd cooling and heating cycle with a cooling/heating rate of 0.15 K/min. The arrows indicate the direction of temperature increase/decrease for each measurement.

# References

(1) Neidhardt, M. M.; Schmitt, K.; Baro, A.; Schneider, C.; Bilitewski, U.; Laschat, S. Self-assembly and biological activities of ionic liquid crystals derived from aromatic amino acids. *Phys. Chem. Chem. Phys.* **2018**, *20*, 20371–20381.

(2) Azefu, Y.; Tamiaki, H.; Sato, R.; Toma, K. Facile synthesis of stable lipid analogues possessing a range of alkyl groups: application to artificial glycolipids. *Bioorganic and Medicinal Chemistry* **2002**, *10*, 4013–4022.

(3) Rosen, B. M.; Peterca, M.; Morimitsu, K.; Dulcey, A. E.; Leowanawat, P.; Resmerita, A.-M.; Imam, M. R.; Percec, V. Programming the Supramolecular Helical Polymerization of Dendritic Dipeptides via the Stereochemical Information of the Dipeptide. *Journal of the American Chemical Society* **2011**, *133*, 5135–5151, PMID: 21391688.
